# Supplementary material for: Ultrafast dynamics of spin and orbital correlations in quantum materials: an energy- and momentum-resolved perspective
Source: arXiv:1809.06288 ancillary file (2018-10-31)
Supplement: Supplementary file 1 [file supplementary_materials.pdf]

# Ultrafast dynamics of spin and orbital correlations in quantum materials: An energy- and momentum-resolved perspective Supplementary material

Y. Cao,<sup>1,2</sup> D. G. Mazzone,<sup>3</sup> D. Meyers,<sup>1</sup> J. P. Hill,<sup>3</sup> X. Liu,<sup>4</sup> S. Wall,<sup>5</sup> and M. P. M. Dean<sup>1</sup>

<sup>1</sup>*Condensed Matter Physics and Materials Science Department,  
Brookhaven National Laboratory, Upton, New York 11973, USA*

<sup>2</sup>*Materials Science Division, Argonne National Laboratory, Argonne, Illinois 60439, USA*

<sup>3</sup>*National Synchrotron Light Source II, Brookhaven National Laboratory, Upton, New York 11973, USA*

<sup>4</sup>*School of Physical Science and Technology, ShanghaiTech University, Shanghai 201210, China*

<sup>5</sup>*ICFO-Institut de Ciències Fotòniques, The Barcelona Institute of  
Science and Technology, 08860 Castelldefels (Barcelona), Spain*

This supplementary information contains a brief introduction to RIXS Spectrometers and the factors that contribute to their energy resolution.

## RIXS SPECTROMETER IN THE SOFT X-RAY REGIME

The general purpose of an X-ray spectrometer is to spatially separate X-ray photons of different energies. In the case of soft X-rays, the principle optical elements tend to be grazing incidence diffraction gratings. The dispersed soft X-ray photons are subsequently focused onto a position sensitive detector, which is usually achieved either with a single concave grating, or a combination of a focusing mirror and a plane grating. Two-element setups tend to be easier to manufacture to very tight tolerances, but may be more complicated to align and prone to mechanical or thermal instabilities when compared to single element setups. To serve special purposes and to meet particular mechanical or scientific requirements, more complicated X-ray optical designs start to be considered.

The key factors that affect the energy resolution of soft X-ray spectrometers are (1) the length of the spectrometer arm; (2) the X-ray beam footprint along the energy dispersing direction; and (3) the spatial resolution of the X-ray detector. There are other contributing factors, such as the grating slope error for the concave grating in the single element setup. The primary factor determining the energy resolution is the length of the spectrometer arm, ranging from several meters up to  $\sim 16$  m [1]. The grating equation for the 1st order diffraction can be written as

$$\frac{hc}{E} = d(\sin \alpha + \sin \beta). \quad (1)$$

The contributions to the spectrometer energy resolution arising from a finite source with size  $S_1$  and a finite detector pixel size  $S_2$  are respectively

$$\Delta E_{S_1} = (E^2/hc)d \cos \alpha S_1/r_1 \quad (2)$$

$$\Delta E_{S_2} = (E^2/hc)d \cos \beta S_2/r_2 \quad (3)$$

with the total resolution being the vector summation.  $\alpha$ ,  $\beta$ ,  $r_1$  and  $r_2$  are as defined in Fig. 1(a), and  $d$  is the grating average groove distance. In the soft X-ray range, photons scattered from the sample arrive at grazing angles relative to the grating, with  $\alpha$  close to  $90^\circ$  and  $\beta$  close to  $-90^\circ$ . At the Cu  $L_3$  edge ( $h\nu \sim 930$  eV), an effective detector pixel size of  $S_2 = 10 \mu\text{m}$  at  $r_2 = 3$  m will contribute  $\sim 73$  meV to the energy resolution for a typical line spacing of  $\sim 2500/\text{mm}$  and  $|\beta| \sim 85.5^\circ$ . The contribution from a finite sample source can be estimated accordingly. Notably, the energy resolution from the above calculations simply derives from the grating equation, and is usually underestimated compared with the full simulation. It does not address the specific types of grating, nor does it take into account the role of the focusing mirror, the aberration and many other factors.

## RIXS SPECTROMETER IN THE HARD X-RAY REGIME

Hard X-ray RIXS spectrometers mainly utilize the Bragg diffraction of high quality single crystals, mostly silicon (Si), but also quartz and germanium (Ge). As shown in Fig. 1(b), the X-ray source (sample), the analyzer crystal and the area photodetector are placed in a Rowland geometry. Photons scattered from the sample are collected by the analyzer crystal and refocused onto the detector. A two-dimensional array of analyzer crystals are used to increase

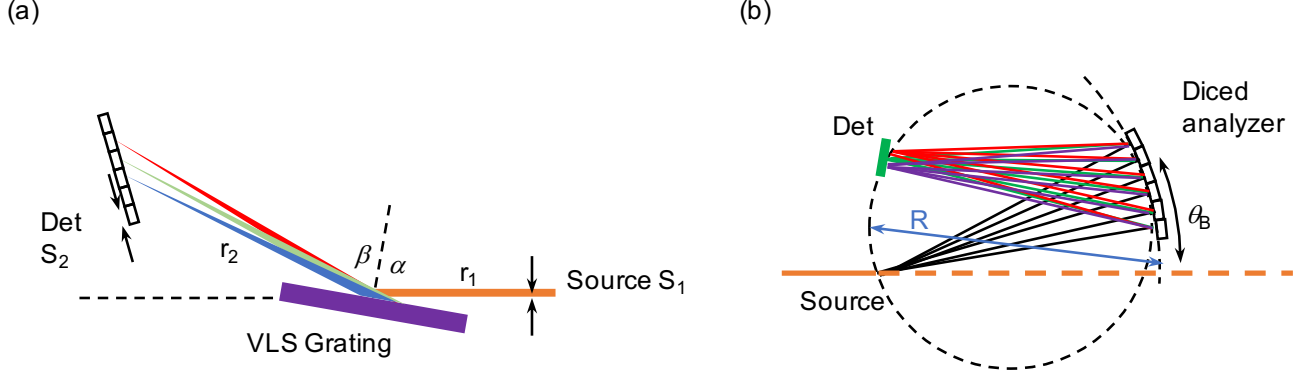

FIG. 1. Schematics of RIXS spectrometers in the (a) soft X-ray and (b) hard X-ray regimes. Panels (a) and (b) are modified from those in Refs. 2 and 3 respectively. “Det” stands for (pixelated) “detector” and “VLS” is the abbreviation for “variable line spacing”. Other notations are introduced in the text.

the photon efficiency. They are placed on a concave plane matching the radius of the Rowland circle, and are often referred to as the ‘diced-and-bent’ analyzers [3]. The energy resolution of the spectrometer is determined by (a) the intrinsic broadening of the single crystal (the Darwin width  $W_D$ ), the geometrical energy resolution (b) arising from a finite photon footprint  $S_1$  on the sample, and (c) from the finite detector pixel size  $S_2$ . Specifically the energy resolution could be estimated as [3]

$$\Delta E_D = W_D E \cot \theta_B \quad (4)$$

$$\Delta E_{S_1} = E \cot \theta_B S_1 / R \quad (5)$$

$$\Delta E_{S_2} = E \cot \theta_B S_2 / 2R. \quad (6)$$

$W_D$ ,  $\theta_B$  and  $R$  are the Darwin width, the Bragg angle of the analyzer crystal and the Rowland radius, respectively. The total spectrometer resolution constitutes from their vector sum. Since the energy resolution improves as  $\theta_B$  approaches  $90^\circ$ , the analyzer crystals are often chosen to work in a nearly-backscattering configuration.

At 11.215 keV (Ir  $L_3$  edge), the Darwin width is  $17.4 \mu\text{rad}$  for the Si (8, 4, 4) reflection. With an 1 m arm and  $S_1 = S_2 = 50 \mu\text{m}$ , the total resolution settles around 49 meV. For typical synchrotrons and free electron lasers, the default photon polarization is horizontal. The elastic line intensity in a RIXS spectrum can be suppressed using a horizontal scattering plane with the spectrometer placed close to  $90^\circ$  relative to the incident X-ray. The X-ray photons scattered from the analyzer crystals are dispersed vertically similar to the setup in the soft X-ray range. We note that it is not required to put the spectrometer close to  $90^\circ$  when using soft X-rays.

Recently new energy analyzing schemes aiming at higher energy resolutions or photon efficiencies have been proposed and/or demonstrated [4–8], so the above estimates may be surpassed in future tr-RIXS setups.

- 
- [1] Dvorak J, Jarrige I, Bisogni V, Coburn S, and Leonhardt W. 2016 Towards 10 meV resolution: The design of an ultrahigh resolution soft X-ray RIXS spectrometer. *Rev. Sci. Instr.* **87**, 115109.
  - [2] Ghiringhelli G, Piazzalunga A, Dallera C, Trezzi G, Braicovich L, Schmitt T, Strocov VN, Betemps R, Patthey L, Wang X, et al. 2006 SAXES, a high resolution spectrometer for resonant x-ray emission in the 400–1600 eV energy range. *Rev. Sci. Instr.* **77**, 113108.
  - [3] Shvyd'ko YV, Hill JP, Burns CA, Coburn DS, Brajuskovic B, Casa D, Goetze K, Gog T, Khachatryan R, Kim JH, et al. 2013 MERIX-next generation medium energy resolution inelastic X-ray scattering instrument at the APS. *J. Electron Spectros. Relat. Phenomena* **188**, 140–149.
  - [4] Chuang YD, Anderson C, Benk M, Goldberg K, Voronov D, Warwick T, Yashchuk V, and Padmore H. 2016 Multiplexed high resolution soft x-ray RIXS. In *AIP Conference Proceedings*, volume 1741, p. 050011. AIP Publishing.
  - [5] Chuang YD, Shao YC, Cruz A, Hanzel K, Brown A, Frano A, Qiao R, Smith B, Domning E, Huang SW, et al. 2017 Modular soft x-ray spectrometer for applications in energy sciences and quantum materials. *Rev. Sci. Instr.* **88**, 013110.
  - [6] Kim J, Shi X, Casa D, Qian J, Huang X, and Gog T. 2016 Collimating Montel mirror as part of a multi-crystal analyzer system for resonant inelastic X-ray scattering. *Journal of synchrotron radiation* **23**, 880–886.

- [7] Kim J, Casa D, Said A, Krakora R, Kim BJ, Kasman E, Huang X, and Gog T. 2018 Quartz-based flat-crystal resonant inelastic X-ray scattering spectrometer with sub-10 meV energy resolution. Sci. Rep. **8**, 1958.
- [8] Shvydko Y. 2016 X-ray echo spectroscopy. Phys. Rev. Lett. **116**, 080801.
